# Supplementary material for: A microfluidic band-pass filter for flexible fiber separation
Source: arXiv:2508.19166 ancillary file (2026-01-13)
Supplement: Supplementary file 1 [file SI_pdf.pdf]

# Supporting Information for

## A microfluidic band-pass filter for flexible fiber separation

**Zhibo Li, Clément Bielinski, Anke Lindner, Blaise Delmotte and Olivia du Roure**

**Corresponding Authors: Anke Lindner, Blaise Delmotte and Olivia du Roure.**
**E-mail: anke.lindner@espci.fr, blaise.delmotte@cnrs.fr, olivia.duroure@espci.fr**

### This PDF file includes:

Supporting text
Figs. S1 to S3
Legends for Movies S1 to S3

### Other supporting materials for this manuscript include the following:

Movies S1 to S3

# Supporting Information Text

## 1. Chip-scale experimental setup

Fig. S1 illustrates the chip-scale experimental setup designed to investigate fiber suspension separation and the bandpass effect at the optimal flow angle, $\alpha = 35°$. This setup features a wider channel ($W_{\mathrm{array}} = 2000\,\mu\mathrm{m}$) and an extended pillar array region ($L_{\mathrm{array}} = 12\,\mathrm{mm}$, partially shown in the sketch) while maintaining the same pillar layout. Through flow focusing, the buffer flow rate, $Q_2$, is set to be 20 times that of the dilute actin filament suspension, $Q_1$, ensuring that the suspension (green) enters the array as a narrow band near the wall. The fibers are then transported downstream within the array. To analyze their lateral drift, we count the number of fibers further downstream at $x_{\mathrm{obs}} = 6\,\mathrm{mm}$ at the mid-height plane of the channel and measure their lengths at various lateral positions, $y_{\mathrm{obs}}$, relative to the wall. The drift angle of each fiber is then estimated as $\beta = \arctan(y_{\mathrm{f}}/x_{\mathrm{f}})$, where the subscript f indicates the fiber's final position at the time the images are recorded.

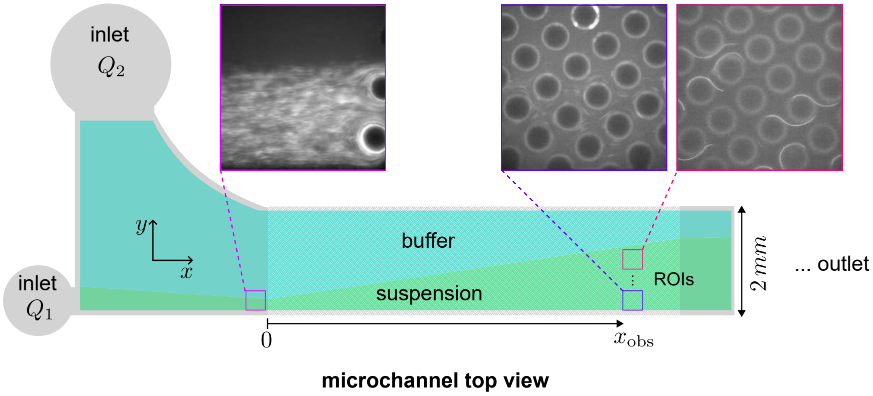


**Fig. S1.** Chip-scale experimental setup. The channel has two inlets: one for delivering the actin filament suspension at a flow rate of $Q_1$, and another for the buffer at $Q_2 = 20Q_1$. The observation windows (ROIs) are positioned at $x_{\mathrm{obs}} = 6\,\mathrm{mm}$ from the start of the array and are sequentially shifted along the $y$-direction. Three representative experimental snapshots at different positions are presented above. The concentration of filament suspension is $50\,\mathrm{nM}$.

## 2. Flow lanes analysis

As shown in Fig. S2, when a fiber wraps around pillar $P_{\mathrm{n}}$, the widths of the flow lanes (depicted in blue and red) between pillars $P_{\mathrm{n+1}}$ and $P_{\mathrm{n+3}}$ play a crucial role in fiber separation. We estimate these widths, $w_1$ and $w_2$, based on the periodic nature of the flow.

Since the channel depth is five times larger than the gaps between adjacent pillars, and measurements are taken at the channel's mid-height plane, we assume parabolic flow profiles between the gaps:

$$u_1 = k_1 x^2 - k_1 x \qquad u_2 = k_2 y^2 - k_2 y \tag{1}$$

By applying mass conservation, we obtain

$$\int_0^1 u_1\,dx = \int_0^{w_1+w_2} u_2\,dy \qquad \int_0^1 u_1\,dx + \int_0^{w_1} u_2\,dy = \int_0^1 u_2\,dy \tag{2}$$

Additionally, for a given channel length, the pressure drop remains constant. According to the Hagen–Poiseuille law, the ratio of the maximum velocities at $x = \frac{1}{2}$ and $y = \frac{1}{2}$ is given by

$$u_1(\frac{1}{2})/u_2(\frac{1}{2}) = \tan\alpha \tag{3}$$

Solving this system of equations and selecting reasonable solutions, we determine the widths $w_1$ and $w_2$ at different flow angles $\alpha$, as shown in the right panel of Fig. S2.

 Zhibo Li, Clément Bielinski, Anke Lindner, Blaise Delmotte and Olivia du Roure

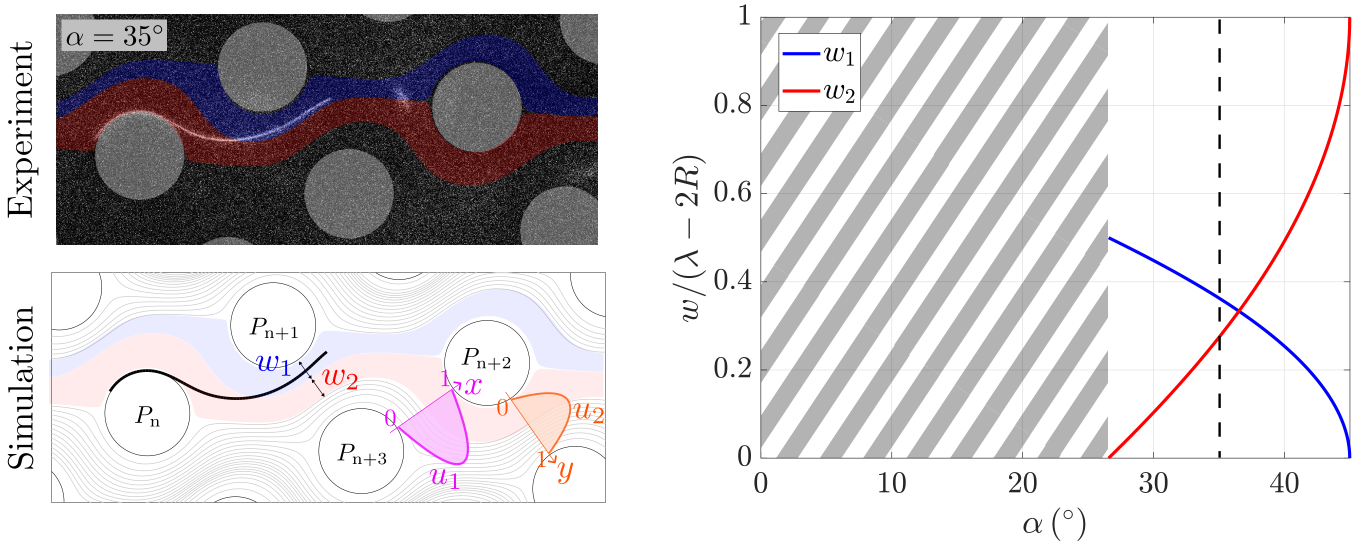


**Fig. S2.** Widths of flow lanes between pillar $P_{n+1}$ and pillar $P_{n+3}$ at various flow angles, as illustrated in the left panels from experimental and numerical snapshots. The gray diagonal line indicates that there is no such flow separation at those flow angles. The dashed line is $\alpha = 35°$.

## 3. The design of precise fiber suspension separation device

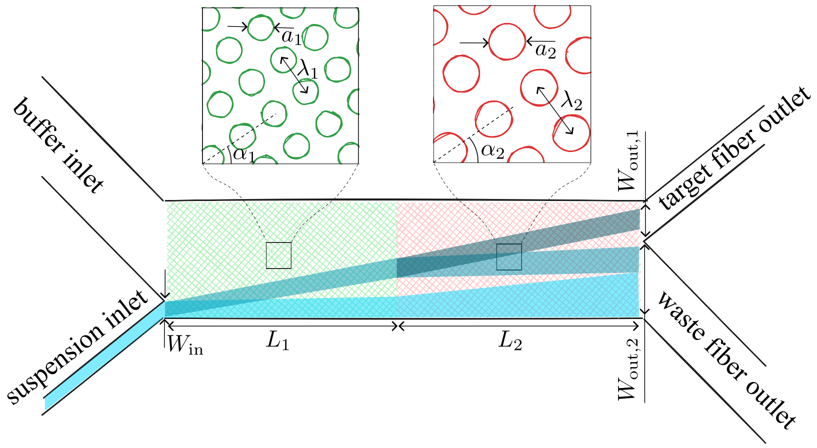


**Fig. S3.** Sketch of precise fiber suspension separation device. The device features two distinct pillar array arrangements. Each array is characterized by a flow angle of $\alpha = 35°$ and a center-to-center distance to pillar diameter ratio of $\lambda_1/a_1 = \lambda_2/a_2 \approx 1.5$. The first array has a length $L_1$ and pillar diameter $a_1$, while the second array has a length $L_2$ and a larger pillar diameter $a_2 > a_1$. The device includes two inlets: one for delivering the suspension with a width of $w_{\mathrm{in}}$, and another for introducing a buffer fluid to focus the suspension into a narrow band. It also has two outlets: one for collecting the target fibers with a width of $w_{\mathrm{out},1}$, and the other for expelling wastes with a width of $w_{\mathrm{out},2}$. The geometry of the device adheres to the following constraints: $L_1\ \tan(8°)\ >\ \max\big(L_1\ \tan(4°) + w_{\mathrm{in}},\ 2\,w_{\mathrm{in}}\big)$ and $(L_1 + L_2)\ \tan(8°)\ >\ w_{\mathrm{out},2}\ >\ L_1\ \tan(8°) + w_{\mathrm{in}} + L_2\ \tan(4°)$. By adjusting the pillar sizes, the device can be optimized to separate fibers of desired lengths based on the findings of the current study.

Fig. S3 illustrates a two-stage deterministic lateral displacement (DLD) device designed to implement the bandpass effect identified in this study for flexible fiber separation. Each stage consists of a tilted pillar array at $\alpha = 35°$ with a constant pillar spacing-to-diameter ratio $\lambda_i/a_i \approx 1.5$ $(i = 1, 2)$. In the first array (length $L_1$, pillar diameter $a_1$), fibers whose contour lengths fall within the first intermediate range ("band 1") are laterally displaced into a side stream, whereas all other fibers undergo only minimal lateral deviation. Downstream, the second array (length $L_2$, pillar diameter $a_2 > a_1$) targets a different intermediate length window ("band 2"), causing fibers within that band to be displaced laterally, while others' lateral displacements are limited. Because only fibers whose lengths lie in the intersection of band 1 and band 2 are deflected by both arrays, they alone are routed into the target outlet. Two inlets—a sample inlet of width $w_{\mathrm{in}}$ and a sheath buffer inlet—hydrodynamically focus the fibers into a narrow band when entering the first array; two outlets (widths $w_{\mathrm{out},1}$ for target and $w_{\mathrm{out},2}$ for waste) collect the separated fractions.

To ensure clear separation, the array dimensions and channel widths satisfy:

$$L_1\ \tan(8°)\ >\ \max\big(L_1\ \tan(4°) + w_{\mathrm{in}},\ 2\,w_{\mathrm{in}}\big) \quad [4]$$

$$(L_1 + L_2)\ \tan(8°)\ >\ w_{\mathrm{out},2}\ >\ L_1\ \tan(8°) + w_{\mathrm{in}} + L_2\ \tan(4°) \quad [5]$$

These inequalities guarantee that only fibers within the intersecting bandpass window are deflected sufficiently to enter the target-fiber outlet, while all undesired fibers are directed into the waste outlet. By selecting those geometrical parameters, the device realizes a tunable and precise bandpass filter for separating flexible fibers by contour length.

**Movie S1. A short fiber of length $L = 0.32\lambda$ in a pillar array at a flow angle $\alpha = 35°$ in experiment (upper panel) and its simulation counterpart (lower panel). The flow direction is from left to right throughout.**

**Movie S2. An intermediate fiber of length $L = 1.60\lambda$ in a pillar array at a flow angle $\alpha = 35°$ in experiment (upper panel) and its simulation counterpart (lower panel).**

**Movie S3. A long fiber of length $L = 3.57\lambda$ in a pillar array at a flow angle $\alpha = 35°$ in experiment (upper panel) and its simulation counterpart (lower panel).**
